# Supplementary material for: Is Fine-tuning Needed? Pre-trained Language Models Are Near Perfect for Out-of-Domain Detection
Source: arXiv:2305.13282 source file (2023-05-22)
Supplement: Supplementary file 1 [file Metrics-for-OOD-Detection.tex]

\section{Metrics for OOD Detection}
\label{sec:appendix-ood-metrics}

Following~\cite{hendrycks2018deep}, we treat OOD samples as the positive class and evaluate detection performance using three metrics: area under the receiver operating characteristic curve (AUROC), the false positive rate at 95\% recall (FPR95) and the area under the precision-recall curve (AUPR). The AUROC roughly aligns to the probability that an OOD sample is given a higher score than an ID one; thus a higher AUROC is better and an uninformative detector has an AUROC of 50\%. The FPR95 metric indicates the probability that an ID sample is incorrectly classified as OOD when 95\% of OOD samples are detected, and thus a lower FPR95 is better.
