# Supplementary material for: Is Fine-tuning Needed? Pre-trained Language Models Are Near Perfect for Out-of-Domain Detection
Source: arXiv:2305.13282 source file (2023-05-22)
Supplement: Supplementary file 2 [file When-is-Mahalanobis-Effective.tex]

\section{When is Mahalanobis Effective?}
\label{sec:appendix-maha-analysis}

The Mahalanobis distance is a metric measuring the distance of a point from a distribution, as is especially accurate in measuring distances in multivariate space with high correlations between features. It projects the data into a space where the correlations are removed, by normalizing covariance between features to 1, and then calculates the Euclidean distance in that space. Strong correlations between features are common with out-of-domain shifts\sltodo{why necessarily so? I worry this paragraph is not well supported either in theory or empirical evidence. Shall we leave this out for now?}, making Mahalanobis distance a more accurate distance metric in these settings.
